# Supplementary material for: Dependence of nuclear spin singlet lifetimes on RF spin-locking power
Source: arXiv:1201.1482 ancillary file (2012-01-06)
Supplement: Supplementary file 1 [file JMR_supp.pdf]

# Supplementary Information: Dependence of nuclear spin singlet lifetimes on RF spin-locking power

Stephen J. DeVience[a], Ronald L. Walsworth[b,c], Matthew S. Rosen[c,d,e]

[a] Department of Chemistry and Chemical Biology, Harvard University, 12 Oxford St., Cambridge, MA 02138

[b] Harvard-Smithsonian Center for Astrophysics, 60 Garden St., Cambridge, MA 02138

[c] Department of Physics, Harvard University, 17 Oxford St., Cambridge, MA 02138

[d] Harvard Medical School, 25 Shattuck Street, Boston, MA 02115

[e] Martinos Center for Biomedical Imaging, 149 Thirteenth St., Charlestown, MA 02129

## S1. Long-Lived Coherence Relaxation

The maximum lifetime of the long-lived coherence (LLC) under zero RF spin-locking power can be found using the conventional two-spin dipole-dipole relaxation model of Solomon [1, 2], which predicts that in most cases $T_{LLC} = 3T_1$. Demonstration of this relation is accomplished by comparing the long-lived coherence experiment with a standard inversion recovery experiment. In the latter case the system is initialized to the state $I_{1Z}(0) = I_{2Z}(0) = -M_0$, where $I_{nZ}(t)$ is the magnetization of nucleus $n$ at time $t$, and $M_0$ is the magnetization of the spins at thermal equilibrium. The Bloch equations then describe the magnetization as a function of time with two relaxation rates, $\rho$ and $\sigma$:

$$I_Z = M_0 \left[1 - 2\exp\left[-(\rho+\sigma)t\right]\right]. \tag{S1}$$

These two relaxation rates are the result of zero, single, and double quantum transitions with rates $W_0$, $W_1$ and, $W_2$ respectively:

$$\begin{aligned} \sigma &= W_2 - W_0 \\ \rho &= W_0 + 2W_1 + W_2. \end{aligned} \tag{S2}$$

The small molecules in this study rotate quickly (GHz rates), and their short correlation times result in transition rates that can be simply related to one another through a constant $k$:

$$k = 10W_0 = 20/3W_1 = 5/3W_2, \tag{S3}$$

where the numerical prefactors for $W_0$, $W_1$ and, $W_2$ are determined from averaging the relative interaction stength of each transition over all angular configurations. Combining equations S1, S2, and S3 allows one to write $T_1$ in terms of k:

$$T_1 = 1/(\rho+\sigma) = \frac{2}{3}\frac{1}{k}. \tag{S4}$$

The long-lived coherence, $\rho_{LLC}$, represents a population difference in the spin-pair eigenbasis:

$$\rho_{LLC} = |\uparrow\downarrow\rangle\langle\uparrow\downarrow| - |\downarrow\uparrow\rangle\langle\downarrow\uparrow| = I_{1z} - I_{2z}. \tag{S5}$$

It results from a selective inversion of the spins rather than the inversion of both spins. The initial conditions for magnetization are $I_{1Z}(0) = -I_{2Z}(0) = M_0$. In this case relaxation is found to be bi-exponential for the individual magnetizations and exponential for the magnetization difference. The Bloch equations for the magnetization of spins one and two are

$$I_{1Z} = M_0 - M_0\exp\left[-(\rho+\sigma)t\right] + M_0\exp\left[(\sigma-\rho)t\right] \tag{S6}$$

$$I_{2Z} = M_0 - M_0\exp\left[-(\rho+\sigma)t\right] - M_0\exp\left[(\sigma-\rho)t\right]. \tag{S7}$$

The difference between these equations describes the magnetization of the long-lived coherence:

$$I_{1Z} - I_{2Z} = 2M_0\exp\left[(\sigma-\rho)t\right]. \tag{S8}$$

This results in a lifetime $T_{LLC} = 1/(\rho-\sigma)$, which can be written in terms of $T_1$ as

$$T_{LLC} = \frac{1}{2(W_0+W_1)} = \frac{2}{k} = 3T_1. \tag{S9}$$

Larger enhancements are possible for the long-lived coherence when the molecules have long correlation times, since the assumptions of equation S3 are no longer valid [3].

## S2. Comparison of Models for Singlet Lifetime Dependence on RF Power

Pileio and Levitt performed exact numerical calculations for the relationship between singlet lifetime and RF power and derived the following equation (eq. 43 in ref. [4] of the supplement):

$$\frac{1}{T_S} \simeq \frac{-b_{jk}^2 \tau_c}{160}[6(4\cos(\theta_\Delta) + \cos(2\theta_\Delta) - 17) + \sqrt{6(281 + 360\cos(\theta_\Delta) + 196\cos(2\theta_\Delta) + 24\cos(3\theta_\Delta) + 3\cos(4\theta_\Delta))}] \tag{S10}$$

where $b_{jk}$ is the dipolar coupling strength, $\tau_c$ is the rotational correlation time of the molecule, and $\theta_\Delta$ is the difference in tilt angles, which is defined as

$$\theta_\Delta = \arctan(\nu_j/\nu_n) - \arctan(\nu_k/\nu_n). \tag{S11}$$

Here, $\nu_n$ is the nutation frequency induced by the RF field, while $\nu_j$ and $\nu_k$ are the resonance frequencies of the two spins. Note that this definition of $\theta_\Delta$ differs from that given in eq. 24 of ref. [4], because eq. 43 requires a measurement of the tilt angle away from the singlet/triplet basis rather than away from the Zeeman basis. Figure S1 compares the results of our simple model and the model of Pileio and Levitt for the dependence of the singlet state lifetime enhancement as a function of $\nu_n$ relative to the chemical shift difference (eq. S10 of the supplement and eq. 18 of the main text) for a maximum singlet lifetime of 10 $T_1$. There is insignificant difference between the results of the two models once $\nu_n > \Delta\nu$ (chemical shift difference).

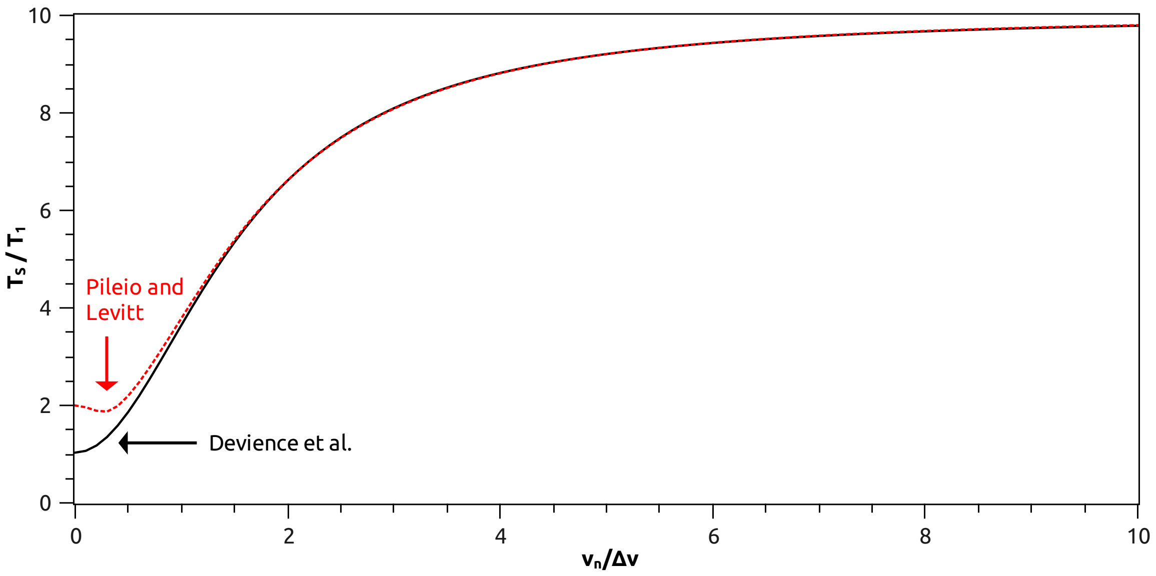


Figure S1: Comparison of the model given by eq. 18 of the main text and eq. 43 of ref. [4] for a singlet with lifetime $T_S = 10\,T_1$. The prefactor $b_{jk}^2\tau_c$ is set to $2/3T_1$, its value in the extreme-narrowing regime. A value of $T_x = 1.15\,T_1$ gives the best agreement between models. The models deviate most at very low RF powers, where higher-order terms become important.

## S3. Temperature Effects

Figure S2 shows measurements for citric acid of the spin-lattice relaxation time $T_1$ and the maximum singlet lifetime $T_S$ at high RF spin-locking power for temperatures between 22 and 54 °C. Both $T_1$ and $T_S$ increase linearly with temperature, and the enhancement ratio $(T_S/T_1)$ changes little over the temperature range. This trend matches previous results [5]. Both $T_1$ and temperature are inversely proportional to the molecular correlation time because in solution small molecules are in the extreme-narrowing regime. Therefore, a linear relationship between $T_1$ and temperature is expected. Since the singlet lifetime is also linear with temperature, we conclude that it must be inversely proportional to correlation time as well, and thus the magnetic quadrupolar interaction is the dominant relaxation mechanism.

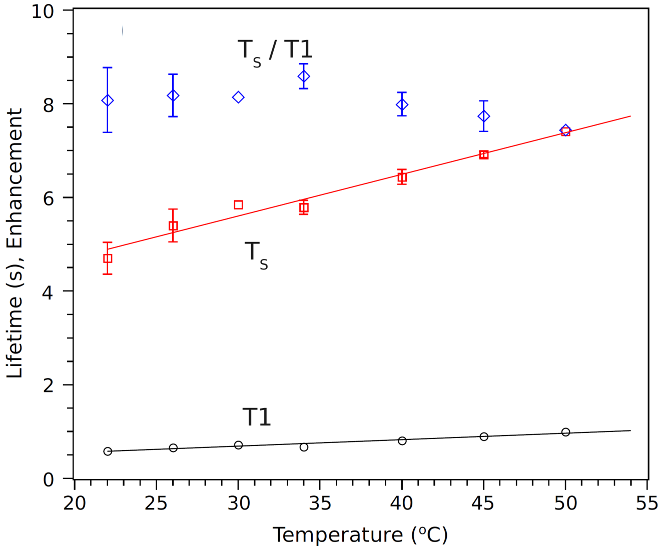


Figure S2: Measured temperature dependences of $T_1$ (black circles) and the maximum singlet lifetime $T_S$ (red squares) are linear for citric acid. ($T_1$ error bars are smaller than symbol size.) Lifetime enhancement ratio $T_S/T_1$ (blue diamonds) has little temperature dependence.

## S4. Pulse Sequences

The long-lived singlet population is prepared most efficiently (up to 50% conversion) via a three-pulse sequence previously described by Levitt and shown in Figure 2A of the main text [6]. The transmit frequency is set between the resonant frequencies of the two protons in the pair. The thermally polarized system is initially in a state $I_{1z} + I_{2z}$. A 90° pulse along x is performed and followed by a delay $\tau_1$, then a 180° pulse and a second delay $\tau_2$, to produce the coherence $2I_{1y}I_{2z} - 2I_{1z}I_{2y}$. This is followed by a 90° pulse along -y, to produce the state $-(2I_{1y}I_{2x} - 2I_{1x}I_{2y}) = i(I_1^+I_2^- - I_1^-I_2^+)$. A final delay $\tau_3$ removes the phase shift and produces $I_1^+I_2^- + I_1^-I_2^+$. This coherence is the population $\rho_{ST} = |T_0\rangle\langle T_0| - |S_0\rangle\langle S_0|$ in the singlet/triplet basis. When $J << \Delta\nu$, the optimal delays are $\tau_1 = 1/(4J)$, $\tau_2 = 1/(4J) + 1/(2\Delta\nu)$, and $\tau_3 = 1/(4\Delta\nu)$. However, in cases where J-coupling is strong, the values must be computed from a model of the system's spin dynamics to take second-order effects into account. We used Levitt's mPackages *Mathematica* program to simulate our systems and approximate optimal values. The mPackages code for Mathematica was programmed by Malcolm H Levitt and Andreas Brinkmann, and is available at www.mhl.soton.ac.uk.

The long-lived coherence (LLC), as well as mixtures of the coherence and the singlet, can be produced via a simpler two-pulse selective inversion sequence shown in Figure 2B of the main text by removing the spin-echo component of Levitt's sequence. After the first 90° pulse along x and the delay $\tau_1$, the proton magnetizations become antialigned along the x-axis of the Bloch sphere. A 90° pulse along -y then creates the population $I_{1z} - I_{2z}$. In the singlet/triplet basis this represents the coherence $\rho_{LLC} = |T_0\rangle\langle S_0| + |S_0\rangle\langle T_0|$. However, J-coupling also leads to the formation of some $i(I_1^+I_2^- - I_1^-I_2^+)$. The second delay, $\tau_2$, can be used to choose the amount of $I_1^+I_2^- + I_1^-I_2^+$, and long-lived singlet population, to mix with the long-lived coherence. Figures S3A and S3B illustrate how the amounts of induced singlet and long-lived coherence oscillate after the final preparatory pulse of each sequence, thereby resulting in different mixtures depending on the time at which the RF spin-locking is first applied.

The RF spin-locking field is applied using CW decoupling for time $\tau_4$. The RF is then turned off and the system is allowed to evolve for a delay $\tau_5$ before a 90° pulse along x is applied and an FID is acquired.

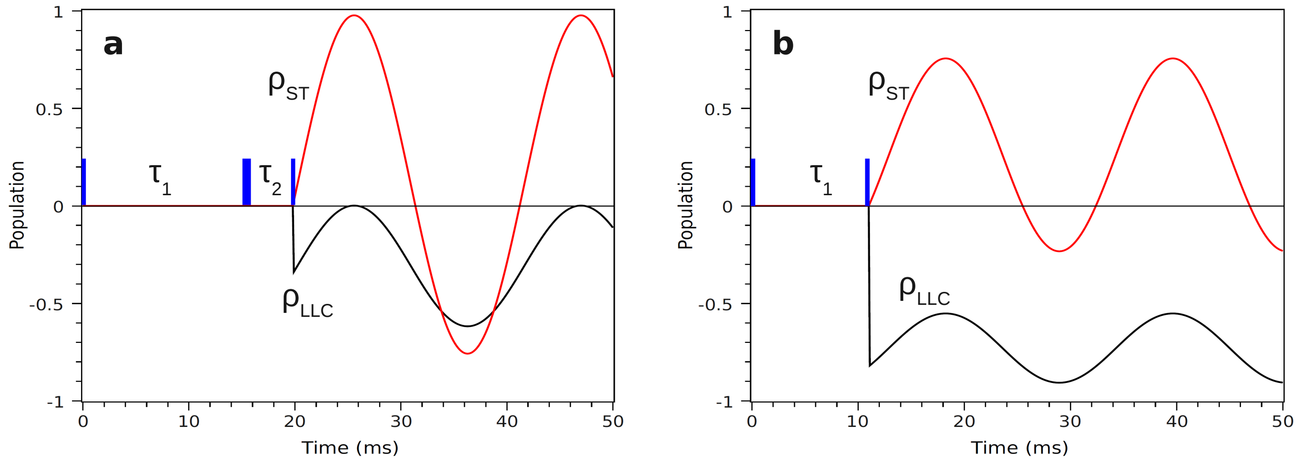


Figure S3: (A) Three-pulse sequence used to prepare the singlet-enhanced superposition $\rho_{ST}$ by choosing the correct values for the delays. After the preparatory pulses, the amount of $\rho_{ST}$ oscillates. (B) Two-pulse sequence used to create either a pure long-lived coherence, $\rho_{LLC}$, or a mixture of $\rho_{LLC}$ and $\rho_{ST}$.

## S5. Effect of Off-Resonance RF Spin-Locking

We found that increased lifetime enhancement ($T_S/T_1$) was achieved in glycerol formal when the RF power was slightly off-resonance. Glycerol formal is special because it exists in two interconverting structures and has overlapping spectral lines. We refer to the peaks from one structure as "a" and "b" and from the other structure as "b" and "c", since the "b" peaks are completely overlapping. Peak "c" was found to have a longer lifetime when the RF transmit frequency was centered between "a" and "b." Table S1 summarizes the measurements made with the RF transmit frequency centered at the two different positions. In Fig. 3C and Table 1 of the main text we present measurements for peak "c" with the RF transmit frequency centered between "b" and "c."

Table S1: Measured values of spin-lattice, singlet, and long-lived coherence relaxation times for glycerol formal.

| RF frequency | Peak | $T_1(s)$ | $T_S(s)$ | Enhancement ($T_S/T_1$) | $T_{LLC}(s)$ | Enhancement ($T_{LLC}/T_1$) |
|---|---|---|---|---|---|---|
| between a & b | a | $0.95 \pm 0.01$ | $1.07 \pm 0.01$ | $1.13 \pm 0.02$ | $1.3 \pm 0.2$ | $1.4 \pm 0.2$ |
| | b | $0.68 \pm 0.01$ | $2.81 \pm 0.03$ | $4.13 \pm 0.08$ | $1.4 \pm 0.2$ | $2.1 \pm 0.3$ |
| | c | $0.68 \pm 0.01$ | $2.09 \pm 0.02$ | $3.07 \pm 0.05$ | $1.12 \pm 0.06$ | $1.65 \pm 0.09$ |
| between b & c | a | $0.95 \pm 0.01$ | $1.30 \pm 0.05$ | $1.37 \pm 0.05$ | $1.14 \pm 0.04$ | $1.20 \pm 0.04$ |
| | b | $0.68 \pm 0.01$ | $2.07 \pm 0.05$ | $3.04 \pm 0.09$ | $1.06 \pm 0.08$ | $1.6 \pm 0.1$ |
| | c | $0.68 \pm 0.01$ | $1.91 \pm 0.03$ | $2.81 \pm 0.06$ | $1.37 \pm 0.02$ | $2.01 \pm 0.04$ |

We also measured the maximum singlet lifetime in citric acid when the transmit frequency of the RF spin-lock was moved away from the average resonance frequency of the proton pair. A theoretical analysis predicts that the relaxation rate should increase quadratically with RF-field offset for relatively small frequency shifts [4, 7]. We set

the RF spin-locking nutation rate to 565 Hz and employed a mixture of singlet and long-lived coherence. As seen in Fig. S4, the measured large-scale increase in relaxation rate is quadratic, but deviations are clearly evident between the lifetimes of each proton of the pair. At RF frequency offsets between 30 and 90 Hz, the relaxation rate decreases for the proton whose resonance frequency is closer to the RF transmit frequency while the relaxation rate of the other proton increases. This trend differs from what we observed in glycerol formal, where we measured a longer singlet lifetime when the RF spin-locking field frequency was moved away from the resonance frequency by 20 Hz.

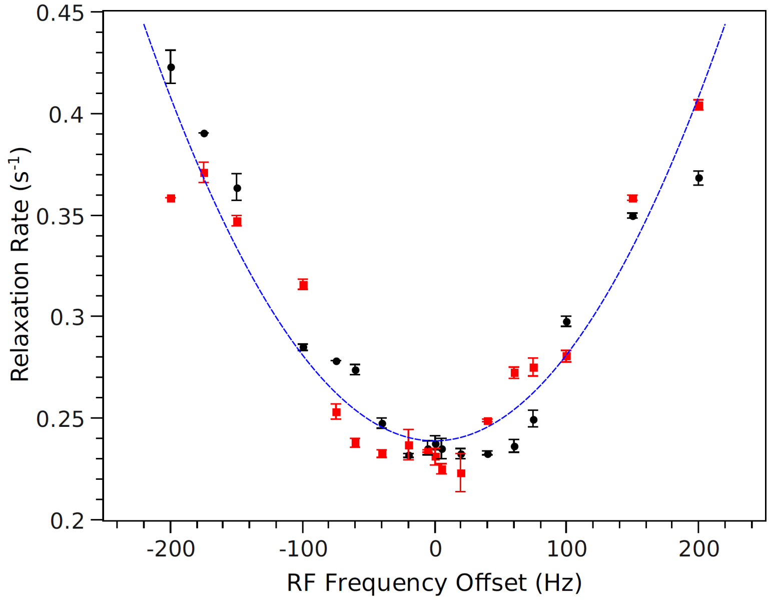


Figure S4: For citric acid prepared with a mixture of singlet population and long-lived coherence, we measured an approximately quadratic relationship between the singlet relaxation rate and the frequency offset of the RF spin-locking field from the average frequency of the proton spin pair. Note the significant deviations between the relaxation rates of the lower-frequency proton (red squares) and the higher-frequency proton (black circles).

## References


[1] I. Solomon, Physical Review 99 (1955) 559–565.

[2] C. P. Slichter, Principles of Magnetic Resonance, Springer-Verlag, Berlin, 1990.

[3] A. Bornet, R. Sarkar, G. Bodenhausen, Journal of Magnetic Resonance 206 (2010) 154–156.

[4] G. Pileio, M. H. Levitt, Journal of Chemical Physics 130 (2009) 214501.

[5] S. Cavadini, J. Dittmer, S. Antonijevic, G. Bodenhausen, Journal of the American Chemical Society 127 (2005) 15744–15748.

[6] M. H. Levitt, Encyclopedia of Magnetic Resonance (2010).

[7] K. Gopalakrishnan, G. Bodenhausen, Journal of Magnetic Resonance 182 (2006) 254–259.
